# Supplementary material for: Scaling of quadratic and linear magnetooptic Kerr effect spectra with L2$_1$ ordering of Co$_2$MnSi Heusler compound
Source: arXiv:2003.09728 ancillary file (2020-03-24)
Supplement: Supplementary file 1 [file Suplementary.pdf]

- **Supplemental Material** -

# Scaling of quadratic and linear magnetooptic Kerr effect spectra with $L2_1$ ordering of $Co_2MnSi$ Heusler compound


Robin Silber,[1,2,3] Daniel Král,[4] Ondřej Stejskal,[2,4] Takahide Kubota,[5] Yasuo Ando,[6] Jaromír Pištora,[1,2] Martin Veis,[4] Jaroslav Hamrle,[4] and Timo Kuschel[3]

[1)] *Nanotechnology Centre, VŠB-Technical University of Ostrava, Ostrava, Czech Republic*

[2)] *IT4Innovations, VŠB-Technical University of Ostrava, Ostrava, Czech Republic*

[3)] *Department of Physics, Bielefeld University, Bielefeld, Germany*

[4)] *Faculty of Mathematics and Physics, Charles University, Prague, Czech Republic*

[5)] *Institute for Materials Research, Tohoku University, Sendai, Japan*

[6)] *Department of Applied Physics, Tohoku University, Sendai, Japan*



(Dated: 21 March 2020)

## I. CONVENTIONS

To describe MOKE in experiment setup and the theoretical description, the following sign conventions are employed[1]. Three Cartesian systems are needed to describe reflection from a sample, one for incident light beam, one for reflected light beam and one for the sample. All those Cartesian systems are right-handed and defined in Fig. S1. All the conventions used are described as follow:

*(i) Time convention.* The electric field vector of an electromagnetic wave is described by negative time convention as $\boldsymbol{E}(\boldsymbol{r},t) = \boldsymbol{E}(\boldsymbol{r})e^{-i\omega t}$, providing permittivity in the form $\varepsilon_{ij} = \Re(\varepsilon_{ij}) + i\Im(\varepsilon_{ij})$, providing imaginary part of the diagonal permittivity $\Im(\varepsilon_{ii}) > 0$.

*(ii) Cartesian referential of the sample.* The Cartesian system describing the sample is the right-handed $\hat{x}$, $\hat{y}$, $\hat{z}$ system, where $\hat{z}$-axis is normal to the surface of the sample, and points into the sample. The $\hat{y}$-axis is parallel with the plane of light incidence and with the sample surface, while its positive direction is defined by the direction of $k_y$, being the $\hat{y}$-component of the wave vector of incident light as shown in Fig. S1. In this system, rotations of the crystallographic structure and magnetization take place.

*(iii) Cartesian referential of light.* We use the right-handed Cartesian system $\hat{s}$, $\hat{p}$, $\hat{k}$ for description of the incident and reflected light beam. The direction of vector $\hat{k}$ defines the direction of propagation of light. Vector $\hat{p}$ lies in the plane of incidence, i.e. a plane defined by incident and reflected beam. The vector $\hat{s}$ is perpendicular to this plane and corresponds to $\hat{x}$. This convention is the same for both incident and reflected beams (Fig. S1).

*(iv) Convention of the Kerr angles.* The Kerr rotation $\theta$ is positive if azimuth $\theta$ of the polarization ellipse rotates clockwise, when looking into the incoming light beam. The Kerr ellipticity $\epsilon$ is positive if temporal evolution of the electric field vector $\boldsymbol{E}$ rotates clockwise when looking into the incoming light beam.

*(v) Convention of rotation of the sample, the magnetization and the optical elements.* The rotation is defined as positive if the rotated vector pointing in the $\hat{x}$ ($\hat{s}$) direction rotates towards the $\hat{y}$ ($\hat{p}$) direction. The sample orientation $\alpha = 0$ corresponds to the Fe[100] direction being parallel to the $\hat{x}$-axis and, when looking at the top surface of the sample, the positive rotation of the sample is clockwise. Likewise, the magnetization direction $\mu = 0$ corresponds to $\boldsymbol{M}$ being in the positive direction of the $\hat{x}$-axis and, when looking at the top surface of the sample, the positive rotation of magnetization $\boldsymbol{M}$ is clockwise. Further, when

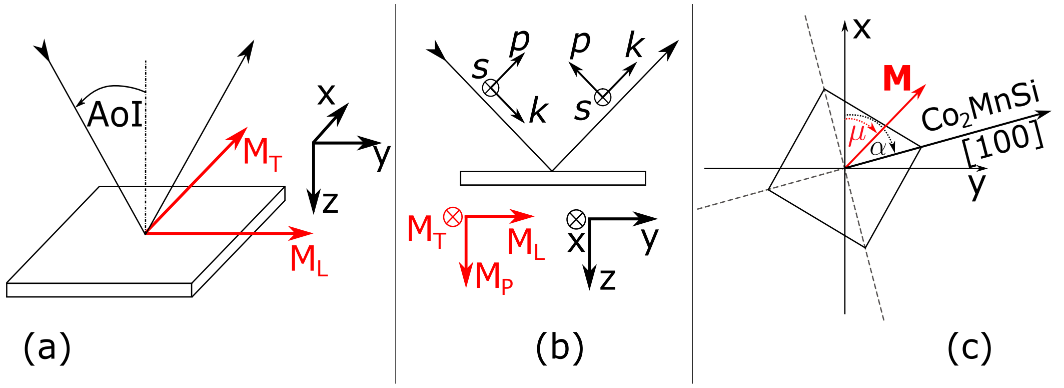


FIG. S1. (a) The right-handed coordinate system $\hat{x}$, $\hat{y}$, $\hat{z}$ is established with respect to the plane of incidence and surface of the sample. Components of the in-plane normalized magnetization $M_T$ and $M_L$ are defined along the axes $\hat{x}$ and $\hat{y}$ of the coordinate system, respectively. (b) Definition of the right-handed Cartesian system $\hat{s}$, $\hat{p}$, $\hat{k}$ of incident and reflected beam. (c) Definition of positive in-plane rotation of the sample and magnetization within the $\hat{x}$, $\hat{y}$, $\hat{z}$ coordinate system, described by angle $\alpha$ and $\mu$, respectively. Figure is based on Fig.1. from Ref.[1]

looking into the incoming beam, the positive rotation of the optical elements is counter-clockwise, in contrast to the positive Kerr angles, defined by historical convention.

## II. MAGNETIC CHARACTERIZATION

In order to successfully separate the QMOKE from the LinMOKE contribution, we have to ensure that our sample is saturated for any magnetization direction. The knowledge of in-plane crystallographic orientation is also crucial to successfully separate QMOKE contribution originating from $G_s$ and $2G_{44}$. In Fig. S2 (a) and (b), we show the magnetic field loops of the samples annealed at 300°C and 500°C respectively. In Fig. S2 (c) the magnetic remanence is plotted against the sample orientation angle $\alpha$. We can see in-plane magnetic easy and hard axes, parallel to $Co_2MnSi\langle 110\rangle$ and $\langle 100\rangle$ directions, respectively, which is in agreement with previous findings[2]). Note that the orientation of magnetic in-plane easy and hard axes do not change upon annealing. Further, the home-build MOKE spectroscopy setup[3] that was used to gather the LMOKE and QMOKE spectra of presented samples utilizes magnetic field of 300 mT, which is clearly more than enough to saturate the sample in any magnetization direction, as a magnetic field of less then 25 mT is already

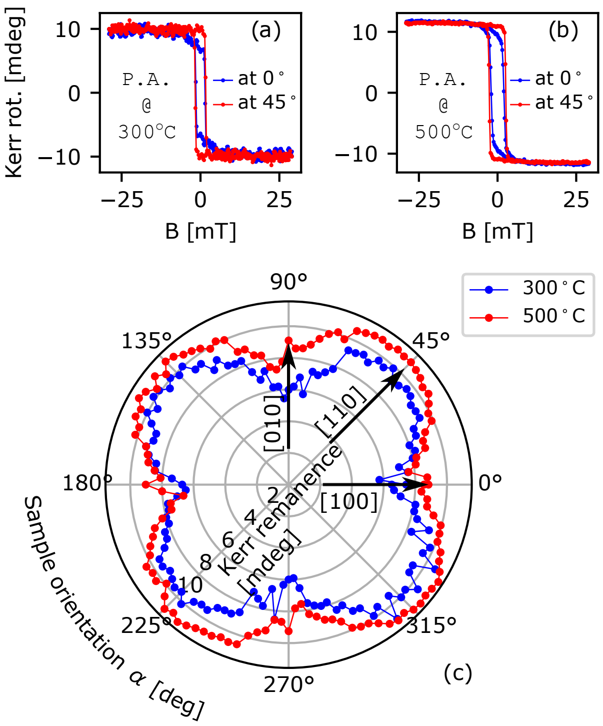


FIG. S2. LMOKE loops of the $Co_2MnSi$ sample that was post annealed at (a) 300°C and (b) 500°C. The loops were symmetrized into odd and even part, only odd part of the loop is shown here. (c) Magnetic remanence of samples annealed at 300°C and 500°C. The crystallographic directions of the $Co_2MnSi$ layer are indicated. The magnetic in-plane easy and hard axes lay in ⟨110⟩ and ⟨100⟩ directions, respectively.

sufficient to saturate each sample in its magnetic in-plane hard axis (Figs. S2 (a) and (b)). All the measurements shown in Fig. S2 were carried out with a light wavelength of 670 nm (≈1.85 eV).

## III. ELLIPSOMETRY

To successfully extract the spectral dependence of MO parameters $K$, $G_s$ and $2G_{44}$, we need to know the spectral dependence of the diagonal permittivity in 0th order $\varepsilon_d$. The optical response of the samples were measured using a dual rotating compensator RC2 Woollam ellipsometer. The measurements were carried out in reflection mode with the angles of incidence 60°, 65°, 70°. Prior to each measurement, the samples were cleaned using UV

spectroscopy-grade (99.8% purity) ethanol. The spectral dependencies of the ellipsometric parameters $\Psi$ and $\Delta$ were obtained in the spectral range of 0.7 eV–6.5 eV. The spectra of $\varepsilon_d$ were calculated from $\Psi$ and $\Delta$ using the Drude model and three Lorentzian oscillators to describe the electron transitions located at approximately 1.7, 1.8 and 5.5 eV. The spectra were processed using CompleteEase[4], an advanced simulation software developed by J. A. Woollam Co., Inc as a software support to the RC2 Woollam ellipsometer.

## IV. THEORETICAL AB-INITIO CALCUALTIONS

The electronic structure of $Co_2MnSi$ was calculated by the Linearized Augmented Plane Wave (LAPW) method using the DFT-based WIEN2k[5] code with a lattice parameter of 5.656 Å. LDA was chosen as the exchange-correlation potential as it performed best (even better than LDA+U) for optical and magnetooptic calculations. The $L2_1$ crystal structure was assumed in all calculations. The electronic structure was calculated with a mesh of 27000 $k$-points in the full Brillouin zone and with the product of the smallest atomic sphere radius and the largest reciprocal space vector set to $R_{\mathrm{MT}}K_{\mathrm{max}} = 7$. The maximum value of partial waves inside the spheres was $l_{\mathrm{max}} = 10$ and the largest reciprocal vector in the charge Fourier expansion was set to $G_{\mathrm{max}} = 12\,\mathrm{Ry}^{\frac{1}{2}}$. These are default values for standard calculations and determine the LAPW basis in which the solution is searched for.

The optical and MO spectra were calculated using the Kubo formula[6,7] on a finer mesh of 216000 $k$-points in the full Brillouin zone. By Lorentz broadening the spectra with $\gamma = 0.5\,\mathrm{eV}$ and applying the Kramers-Kronig relations, the full permittivity tensor is obtained. Only interband contributions to the permittivity tensor are calculated, the conduction electrons contributions (also called Drude term or intraband transitions) are omitted. The calculation was performed for two magnetization directions, namely [100] and [111] relative to the crystallographic axes, in order to acquire the $K$, $G_s$ and $2G_{44}$ spectra directly from the permittivity tensors as[8]

$$K = \frac{1}{2}\left(\varepsilon_{yz}^{([100])} - \varepsilon_{zy}^{([100])}\right), \tag{S1a}$$

$$G_s = \varepsilon_{xx}^{([100])} - \varepsilon_{yy}^{([100])}, \tag{S1b}$$

$$2G_{44} = \frac{3}{2}\left(\varepsilon_{xy}^{([111])} + \varepsilon_{yx}^{([111])}\right), \tag{S1c}$$

where the superscript denotes the magnetization direction relative to the crystal axes.

## REFERENCES


[1]R. Silber, O. Stejskal, L. Beran, L. Cejpek, R. Antoš, T. Matalla-Wagner, J. Thien, O. Kuschel, J. Wollschläger, M. Veis, T. Kuschel, and J. Hamrle, Phys. Rev. B **100**, 043904 (2019).

[2]G. Wolf, J. Hamrle, S. Trudel, T. Kubota, Y. Ando, and B. Hillebrands, "Quadratic magneto-optical Kerr effect in $Co_2MnSi$," J. Appl. Phys. **110**, 043904 (2011).

[3]R. Silber, M. Tomíčková, J. Rodewald, J. Wollschläger, J. Pištora, M. Veis, T. Kuschel, and J. Hamrle, Phot. Nano. Fund. Appl. **31**, 60 (2018).

[4]J. A. Woollam Co., Inc., *CompleteEASE$^{TM}$ Data Analysis Manual* (2008).

[5]P. Blaha, K. Schwarz, G. K. H. Madsen, D. Kvasnicka, and J. Luitz, *WIEN2K, An Augmented Plane Wave + Local Orbitals Program for Calculating Crystal Properties* (Karlheinz Schwarz, Techn. Universität Wien, Austria, 2001).

[6]R. Kubo, J. Phys. Soc. Jpn. **12**, 570–586 (1957).

[7]C. Ambrosch-Draxl and J. O. Sofo, Comput. Phys. Commun. **175**, 1 (2006).

[8]J. Hamrlová, D. Legut, M. Veis, J. Pištora, and J. Hamrle, J. Magn. Magn. Mater. **420**, 143 (2016).
